# Supplementary material for: Self-Supervised Collision Handling via Generative 3D Garment Models for Virtual Try-On
Source: arXiv:2105.06462 source file (2021-05-13)
Supplement: Supplementary file 1 [file appendix.tex]

\begin{appendices}
	\section{Generative Collision-Free Garment Space}
	
	\Igor{\textbf{Practical tips:} if the number of collisions in test is greater than the number of collisions in the randomly sampled points, then increase the weight of the KL divergence. Instead of training with the full loss function since the beginning, start only with the reconstruction loss and very low KL divergence and progressively increase the weight of the other terms. If introducing the collision loss worsens the reconstruction or introduces artifacts, lower the learning rate (i.e., it will fix collisions slower but won't compromise the quality of the results). These are the steps that I followed to find the weights that I use in the final model. They work well for the dress and tshirt, but maybe it's valuable to mention the process that I've followed as 'practical tips' to train our model.}
	
	\Igor{\textbf{Architecture:}  4 dense layers of size 2000 with ReLU activations, layer normalization (not batch normalization) after each activation. Latent space of size 25, I also tried 50 and 100 but they were qualitatively worse and the amount of wrinkles in train was the same. Adam optimizer with learning rate 1e-4 during the first epochs (only optimize reconstruction and KL 0.01) and 1e-5 with full loss.}
	
	\section{Symbols}
	\begin{tabular}{ll}
		$\uptheta$ &  Body pose\\
		$\bar{\uptheta}$ &  Body pose encoded (SoftSMPL)\\
		$\upbeta$ &  Body shape\\
		$\upgamma$ &  Body motion descriptor\\
		$M_\text{B}(\upbeta, \uptheta)$ &  Body skinned mesh\\
		$\mathbf{T}_\text{B}$ & Body template \\
		$M_\text{G}(\upbeta, \uptheta)$ &  Garment skinned mesh\\
		$\mathbf{T}_\text{G}$ & Garment template \\
		$\mathbf{X}$ & Garment deformation in canonical space \\
		$\mathbf{\bar{X}}$ & Garment deformation encoded $\mathbf{\bar{X}}=E(\mathbf{X})$ \\
		$F(\mathbf{X})$ & Deformation gradients of $\mathbf{X}$\\
		$E(\mathbf{X})$ & Garment encoder\\
		$D(\mathbf{\bar{X}})$ & Garment decoder\\
		$R(\upbeta, \upgamma)$ & Garment regressor \\
		$\upepsilon$ & Space between the garment and the body \\
		$W$ & Skinning function \\
		$\mathcal{W}$ & Skinning weights \\
		$J(\upbeta)$ & Skeletal joints \\
	\end{tabular}
\end{appendices}
